# Supplementary material for: STRATA: Simple, Gradient-Free Attacks for Models of Code
Source: arXiv:2009.13562 source file (2021-08-19)
Supplement: Supplementary file 1 [file appendix_notes.tex]

% Optimal thresholds

% dataset proxy
\subsection{Dataset-agnostic black-box attacks}
\label{subsection:dataset_agnostic}

We have now presented the effectiveness of the Goldilocks attack from the frequency of tokens in the training data alone. However, we ask: \textit{do we need the original training data to conduct the attack?} In fact, we find that the Goldilocks attack can generate effective adversarial attacks even without the original training dataset. We can determine token frequency statistics from a different (potentially non-overlapping) surrogate dataset, which could be constructed from publicly available code on sites such as GitHub. We empirically confirm that the Goldilocks attack can use non-overlapping datasets (\javasmall{}, \javamed{}, \javalarge{}) in this way to attack \codetoseq{} models that have been trained on a different Java dataset. We conclude that the token distributions of non-overlapping Java datasets are sufficiently similar for the Goldilocks attack to be effective (Appendix). This confirms that the Goldilocks attack can be applied in a completely black-box setting without knowledge of the model parameters or training dataset.

% limitations
